# Supplementary material for: Relativistic Core-Valence-Separated Molecular Mean-Field Exact-Two-Component Equation-of-Motion Coupled Cluster Theory: Applications to L-edge X-ray Absorption Spectroscopy
Source: arXiv:2506.09008 ancillary file (2025-11-23)
Supplement: Supplementary file 1 [file cvs_si.pdf]

# Supporting Information for "Relativistic Core-Valence-Separated Molecular Mean-Field Exact-Two-Component Equation-of-Motion Coupled Cluster Theory: Applications to L-edge X-ray Absorption Spectroscopy"

Samragni Banerjee,[1] Run R. Li,[2] Brandon C. Cooper,[2] Tianyuan Zhang,[1] Edward F. Valeev,[3, a)] Xiaosong Li,[1, b)] and A. Eugene DePrince III[2, c)]

[1)]*Department of Chemistry, University of Washington, Seattle, WA 98195, USA*

[2)]*Department of Chemistry and Biochemistry, Florida State University, Tallahassee, FL 32306-4390*

[3)]*Department of Chemistry, Virginia Tech, Blacksburg, Virginia 24061, USA*

[a)]Electronic mail: efv@vt.edu

[b)]Electronic mail: xsli@uw.edu

[c)]Electronic mail: adeprince@fsu.edu

## S1. GEOMETRIES AND FROZEN MANIFOLDS FOR MOLECULES

All Cartesian coordinates are in listed angstroms.

### A. $SiCl_4$

Frozen occupied orbitals: 1$s$ and 2$s$ orbitals of both Si and Cl, 2$p$ orbitals of Cl

TABLE S1.

| Atom | $x$ | $y$ | $z$ |
|---|---|---|---|
| Si | 0.000000 | 0.000000 | 0.000000 |
| Cl | 1.192288 | 1.192288 | 1.192288 |
| Cl | -1.192288 | -1.192288 | 1.192288 |
| Cl | 1.192288 | -1.192288 | -1.192288 |
| Cl | -1.192288 | 1.192288 | -1.192288 |

### B. $TiCl_4$

Frozen occupied orbitals: 1$s$ orbitals of both Ti and Cl, 2$s$ orbitals of Ti.
Frozen virtual orbitals: virtual orbitals with energies over $100E_h$.

TABLE S2.

| Atom | $x$ | $y$ | $z$ |
|---|---|---|---|
| Ti | -2.776428 | 0.905225 | 0.000000 |
| Cl | -2.049929 | 1.932622 | 1.779430 |
| Cl | -2.050040 | -1.149545 | 0.000000 |
| Cl | -2.049929 | 1.932622 | -1.779430 |
| Cl | -4.955812 | 0.905200 | 0.000000 |

## C. $VOCl_3$

Frozen occupied orbitals: 1*s* and 2*s* orbitals of both V, O and Cl; 2*p* orbitals of Cl; 3*s* and 3*p* of V.
Frozen virtual orbitals: virtual orbitals with energies over $100E_h$.

TABLE S3.

| Atom | *x* | *y* | *z* |
|---|---|---|---|
| V | -1.019706 | -1.297418 | 0.023988 |
| O | -0.502833 | -0.566553 | 1.289911 |
| Cl | -0.286530 | -0.261024 | -1.701438 |
| Cl | -0.286543 | -3.309881 | 0.058882 |
| Cl | -3.161449 | -1.277060 | 0.059214 |

## D. $CrO_2Cl_2$

Frozen occupied orbitals: 1*s* and 2*s* orbitals of both Cr, O and Cl; 2*p* orbitals of Cl; 3*s* and 3*p* of Cr.
Frozen virtual orbitals: Virtual orbitals with energies over $100E_h$.

TABLE S4.

| Atom | *x* | *y* | *z* |
|---|---|---|---|
| Cr | 0.883574 | -0.134514 | -0.032996 |
| Cl | -1.248453 | -0.150233 | -0.060370 |
| Cl | 1.624035 | 0.865304 | 1.698655 |
| O | 1.401969 | -1.591580 | -0.038326 |
| O | 1.401985 | 0.589432 | -1.297518 |
